# Supplementary material for: Averaging local structure to predict the dynamic propensity in supercooled liquids
Source: arXiv:2105.05921 ancillary file (2021-05-12)
Supplement: Supplementary file 1 [file SupervisedGlassesSI.pdf]

# Supplementary Information
# Averaging local structure to predict the dynamic propensity in supercooled liquids

Emanuele Boattini[1], Frank Smallenburg[2], Laura Filion[1]
[1] *Soft Condensed Matter, Debye Institute of Nanomaterials Science, Utrecht University, Utrecht, Netherlands*
[2] *Université Paris-Saclay, CNRS, Laboratoire de Physique des Solides, 91405 Orsay, France*

## CONTENTS

**Models** 2

**Training configurations** 2

**Structural descriptors** 2
A. Zero-th order descriptors 2
B. Averaged descriptors 3
C. Complete set of descriptors 4

**Training** 4

**Evaluation metrics** 4

**Cutoff radius for the locally averaged descriptors** 4

**Most relevant structural descriptors in the Kob-Andersen system** 4

**Feature selection in the binary hard-sphere mixture** 5

**Predictive power of radial and angular descriptors in the hard-sphere mixture** 6

**References** 6

## MODELS

**Kob-Andersen:** The Kob-Andersen model [1] is a non-additive mixture of 80% (large) $A$ Lennard-Jones (LJ) particles and 20% (small) $B$ LJ particles. The interaction parameters are $\sigma_{BB} = 0.88\sigma_{AA}$, $\sigma_{AB} = 0.8\sigma_{AA}$, $\epsilon_{BB} = 0.5\epsilon_{AA}$, and $\epsilon_{AB} = 1.5\epsilon_{AA}$. The LJ potential is truncated and shifted at a cutoff distance $r_{c,ij} = 2.5\sigma_{ij}$ (where $i, j \in \{A, B\}$), such that the attractive part of the potential is retained.

**Binary hard spheres:** The binary hard-sphere model we consider is a mixture of 30% large $A$ particles and 70% small $B$ particles, with size ratio $\sigma_B/\sigma_A = 0.85$.

## TRAINING CONFIGURATIONS

**Kob-Andersen:** The data set for the Kob-Andersen system is the one from Ref. [2] and consists of a total of 800 equilibrated configurations, which are evenly split into a training and a test set. These configurations were equilibrated by performing molecular dynamics simulations with constant number of particles $N = 4096$, at a state point corresponding to temperature $k_B T/\epsilon_{AA} = 0.44$ with $k_B$ Boltzmann's constant, and pressure $P\sigma_{AA}^3/\epsilon_{AA} = 2.93$. The dynamic propensities were then computed by performing, for each equilibrated configuration, $M = 30$ independent simulations in the microcanonical ensemble, all starting from the same initial configuration, but with random velocities drawn from the Maxwell-Boltzmann distribution. Specifically, the dynamic propensity of particle $i$ after a time interval $t$ is defined as an isoconfigurational ensemble average of its absolute displacement

$$d_i(t) = \langle |\mathbf{r}_i(t) - \mathbf{r}_i(0)| \rangle, \tag{S1}$$

where $\mathbf{r}_i(t)$ is the position of particle $i$ at time $t$, and the average is taken over the independent runs.

**Binary hard spheres:** For the hard-sphere model, we perform event-driven molecular dynamics simulations in the microcanonical ensemble and generate a data set consisting of a total of 100 equilibrated configurations with $N = 2000$ particles and packing fraction $\eta = 0.58$. The dynamic propensity of each particle is then computed as an isoconfigurational ensemble average over $M = 100$ independent runs. Again, half of this data set is used for training, and the other half is used for testing the models.

The hard-sphere snapshots and the associated dynamic propensities are included as as supplementary data file.

## STRUCTURAL DESCRIPTORS

### A. Zero-th order descriptors

To describe the local environment of each particle $i$ in the dataset, we use a combination of radial (density) and angular functions similarly to previous works [2, 3].

For the radial functions, we consider the same type of functions that were used in Refs. [2, 3] in combination with SVMs. These functions essentially measure the density of particles at a distance $r$ from a reference particle $i$ in a shell of width $2\delta$, and are defined as follows:

$$G_i^{(0)}(r, \delta, s) = \sum_{j \neq i : s_j = s} e^{-\frac{(r_{ij} - r)^2}{2\delta^2}} \tag{S2}$$

where $i$ is the reference particle, $r_{ij}$ is the distance between particle $i$ and $j$, $s_j = A, B$ is the species of particle $j$, and $s$ is the species of particles whose density we wish to probe. By varying $r$, $\delta$, and $s$, these functions capture different aspects of the local density around particle $i$.

For the angular functions, inspired by standard bond-orientational order parameters [4], we use a distance-dependent expansion of the local density in terms of spherical harmonics. First, for any given particle $i$, we define the complex quantities

$$q_i^{(0)}(l, m, r, \delta) = \frac{1}{Z} \sum_{j \neq i} e^{-\frac{(r_{ij} - r)^2}{2\delta^2}} Y_l^m(\mathbf{r}_{ij}), \tag{S3}$$

where $Y_l^m(\mathbf{r}_{ij})$ are the spherical harmonics of order $l$, with $m$ an integer that runs from $m = -l$ to $m = +l$, and $Z = \sum_{j \neq i} e^{-\frac{(r_{ij}-r)^2}{2\delta^2}}$ is a normalization constant. Then, rotationally-invariant angular descriptors are defined as

$$q_i^{(0)}(l, r, \delta) = \sqrt{\frac{4\pi}{2l+1} \sum_{m=-l}^{l} |q_i^{(0)}(l, m, r, \delta)|^2}. \tag{S4}$$

These quantities measure the $l$-fold symmetry of the distribution of neighbors at a distance $r$ from a reference particle $i$ in a shell of width $2\delta$.

The full vector $\mathbf{X}_i^{(0)}$ for a given particle $i$ then consists of the values of $G_i^{(0)}(r, \delta, s)$ and $q_i^{(0)}(l, r, \delta)$, evaluated for a fixed set of $r$, $\delta$, and $l$.

For the Kob-Andersen system, we build a set of 200 radial functions by setting $s \in \{A, B\}$, and considering 60 equally spaced distances in the interval $r/\sigma_A \in (0.5, 2.0]$ with $\delta = 0.025$, 20 equally spaced distances in the interval $r/\sigma_A \in (2.0, 3.0]$ with $\delta = 0.05$, and 20 equally spaced distances in the interval $r/\sigma_A \in (3.0, 5.0]$ with $\delta = 0.1$. For the angular functions, we use $\delta = 0.1$, $l \in [1, 12]$, and 16 equally spaced distances in the interval $r/\sigma_A \in [1, 2.5]$, resulting in 192 angular descriptors. Hence, the full vector $\mathbf{X}_i^{(0)}$ for Kob-Andersen has a dimensionality of $D = 392$.

For hard spheres, we use the same parameters but consider only distances larger than $\sigma_B/\sigma_A = 0.85$, resulting in a set with fewer (172) radial functions and a vector $\mathbf{X}_i^{(0)}$ of dimensionality $D = 364$.

### B. Averaged descriptors

In order to incorporate the shell-averaging concept from GNNs, we then introduce higher-order descriptors $\mathbf{X}_i^{(n)}$, where each consecutive $\mathbf{X}_i^{(n)}$ is defined as a local average of the previous order $\mathbf{X}_i^{(n-1)}$. Specifically:

$$\mathbf{X}_i^{(n)} = \frac{1}{C} \sum_{j: r_{ij} < r_c} e^{-r_{ij}/r_c} \mathbf{X}_j^{(n-1)}, \tag{S5}$$

where $r_c$ is a cutoff radius and $C = \sum_{j: r_{ij} < r_c} e^{-r_{ij}/r_c}$.

The results in the main text are obtained using a cutoff distance of $r_c/\sigma_{AA} = 2.3$ for Kob-Andersen and $r_c/\sigma_A = 2.1$ for hard spheres. As shown in Fig. S1, these cutoffs include approximately two shells of neighbours and were chosen as the distance at which the radial distribution function has its second minimum. Note, however, that the final results are only weakly affected by the particular choice of $r_c$.

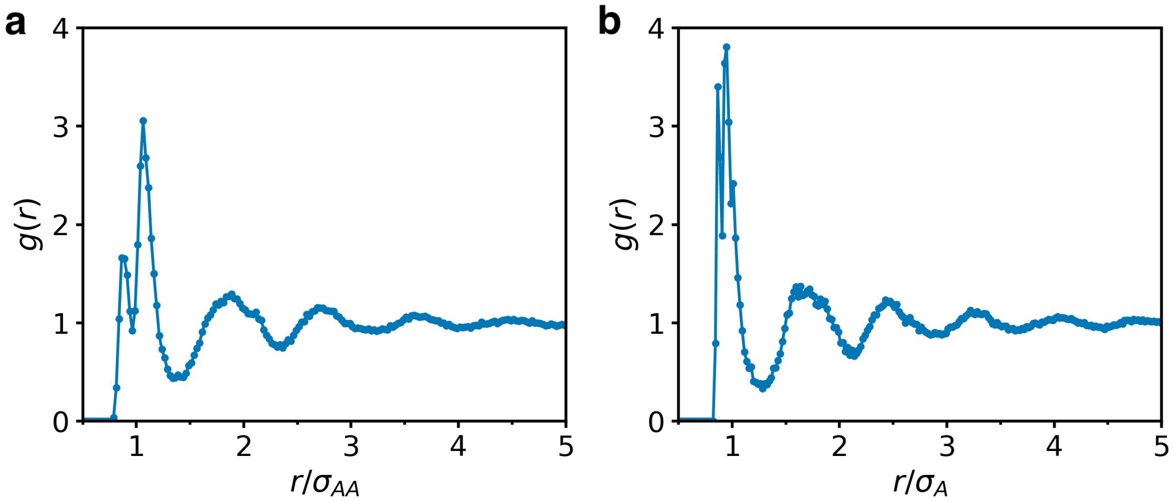


FIG. **S1**: Radial distribution function of a single representative snapshot of the (a) Kob-Andersen and (b) hard-sphere systems.

### C. Complete set of descriptors

We define $\mathcal{X}^{(n_{\max})}$ to be the combination of descriptors (angular and/or radial) from each shell up to a maximum level of $n_{\max}$. Note that in the main text, this set sometimes includes both the angular and radial components, and sometimes one or the other is excluded. In all cases, this is clearly indicated in the text.

## TRAINING

We fit the dynamic propensity of the particles at a given time $t$ as a linear combination of the structural descriptors described in the previous Section, so that our approximation $d_i'$ of the propensity of particle $i$ reads

$$d_i' = w_0 + \sum_{k=1}^{D} w_k x_k, \tag{S6}$$

where $x_k$ is the $k$'th element of the set of descriptors $\mathcal{X}_i^{(n_{\max})}$ for particle $i$, $D$ is the total number of descriptors, and the coefficients $w_k$ are the free parameters of the model. These parameters are optimized by minimizing the sum-of-squares error with the addition of an $L^2$ penalty for the coefficients

$$E(\mathbf{w}) = \sum_{i=1}^{N_t} (d_i - d_i')^2 + \lambda \sum_{k=1}^{D} w_k^2, \tag{S7}$$

where, $\mathbf{w} = (w_0, w_1, \dots, w_D)$, $N_t$ is the total number of particles in the training data set, $d_i$ is the actual propensity of particle $i$ at time $t$, and $\lambda$ is the regularization coefficient. The optimal value of $\lambda$ is found by training several models with different $\lambda$, and finally selecting the model with the smallest error on the test set. Note that before optimizing the parameters of the model, we standardize both the input descriptors and the target propensities so that they have mean zero and unit variance. The optimization of the parameters is performed with the Ridge regression package of the scikit-learn library [5].

## EVALUATION METRICS

To evaluate the performance of our models, we compute the Pearson correlation coefficient between the predicted $d_i'$ and true $d_i$ propensity of all particles in the test set:

$$r_{d'd} = \frac{\sum_{i=1}^{N_t} \left(d_i' - \bar{d}'\right)\left(d_i - \bar{d}\right)}{\sqrt{\sum_{i=1}^{N_t} \left(d_i' - \bar{d}'\right)^2} \sqrt{\sum_{i=1}^{N_t} \left(d_i - \bar{d}\right)^2}}, \tag{S8}$$

where $\bar{d}'$ and $\bar{d}$ are, respectively, the means of the predicted and true propensities.

## CUTOFF RADIUS FOR THE LOCALLY AVERAGED DESCRIPTORS

In this work, we locally average the structural descriptors over a spherical local region that includes approximately the first two shells of neighbours. To do so, we fix the cutoff radius $r_c$ of this spherical region as the distance at which the radial distribution function has its second minimum. Here, we explore how the choice of such a radius influences the performance of the final model. To this end, we compute locally averaged descriptors up to order $n_{\max} = 2$ using three different cutoff radii, corresponding to the first, second, and third minimum of the radial distribution function. We then use these three sets of the descriptors to train three distinct models, and we compare their performance.

A comparison of the results obtained with different cutoff radii for the A particles of the Kob-Andersen system is shown in Fig. S2. In general, we find that the the final results are only weakly affected by the particular choice of $r_c$, with only the smallest cutoff performing slightly worse than the other two.

## MOST RELEVANT STRUCTURAL DESCRIPTORS IN THE KOB-ANDERSEN SYSTEM

In the main text, we have shown that the feature selection procedure introduced in Ref. 6 could be used to select a limited set of structural descriptors to accurately predict the dynamic propensity at a given time. In Tab. I, we give the list of the first 20 descriptors selected for predicting the dynamic propensity at $t = \tau_\alpha$ of the A particles of the Kob-Andersen system.

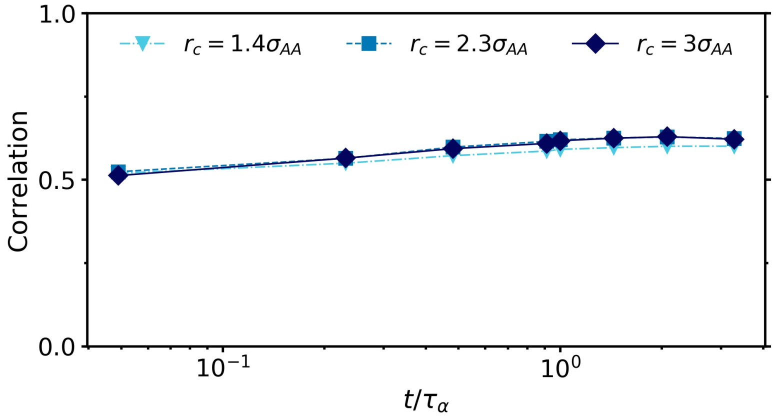


FIG. **S2**: Pearson correlation coefficient between predicted and actual propensities for the $A$ particles of the KA system obtained with three different models. Each model is trained using descriptors which are locally averaged over a spherical region with a different cutoff radius $r_c$.

| index | descriptor |
|---|---|
| 1 | $q^{(2)}(r = 1.700, \quad \delta = 0.100, \quad l = 8)$ |
| 2 | $q^{(2)}(r = 1.000, \quad \delta = 0.100, \quad l = 3)$ |
| 3 | $G^{(2)}(r = 1.400, \quad \delta = 0.025, \quad s = A)$ |
| 4 | $q^{(2)}(r = 1.000, \quad \delta = 0.100, \quad l = 2)$ |
| 5 | $q^{(2)}(r = 1.300, \quad \delta = 0.100, \quad l = 9)$ |
| 6 | $q^{(2)}(r = 1.700, \quad \delta = 0.100, \quad l = 7)$ |
| 7 | $q^{(0)}(r = 1.100, \quad \delta = 0.100, \quad l = 5)$ |
| 8 | $q^{(2)}(r = 1.200, \quad \delta = 0.100, \quad l = 12)$ |
| 9 | $G^{(0)}(r = 2.400, \quad \delta = 0.050, \quad s = A)$ |
| 10 | $q^{(2)}(r = 1.800, \quad \delta = 0.100, \quad l = 9)$ |
| 11 | $q^{(2)}(r = 1.300, \quad \delta = 0.100, \quad l = 10)$ |
| 12 | $G^{(2)}(r = 1.475, \quad \delta = 0.025, \quad s = A)$ |
| 13 | $q^{(2)}(r = 1.500, \quad \delta = 0.100, \quad l = 2)$ |
| 14 | $q^{(2)}(r = 1.000, \quad \delta = 0.100, \quad l = 4)$ |
| 15 | $G^{(2)}(r = 1.125, \quad \delta = 0.025, \quad s = B)$ |
| 16 | $q^{(2)}(r = 1.000, \quad \delta = 0.100, \quad l = 6)$ |
| 17 | $q^{(2)}(r = 1.200, \quad \delta = 0.100, \quad l = 3)$ |
| 18 | $q^{(2)}(r = 1.300, \quad \delta = 0.100, \quad l = 11)$ |
| 19 | $G^{(0)}(r = 3.700, \quad \delta = 0.100, \quad s = A)$ |
| 20 | $q^{(2)}(r = 1.000, \quad \delta = 0.100, \quad l = 12)$ |

TABLE I: List of the first 20 descriptors selected for maximizing the correlation with the dynamic propensity (at $t = \tau_\alpha$) of A particles in the Kob-Andersen system. The index indicates the order of selection.

## FEATURE SELECTION IN THE BINARY HARD-SPHERE MIXTURE

As done for the KA system, we employ the feature selection scheme from Ref. 6 in order to find an optimal subset of descriptors that can accurately predict the dynamics in the case of binary hard spheres. In Fig. S3, we report the results of the predictions at $t = \tau_\alpha$ as a function of the number of selected descriptors. Impressively, after only $N_s = 20$ descriptors have been selected, the accuracy essentially stops improving.

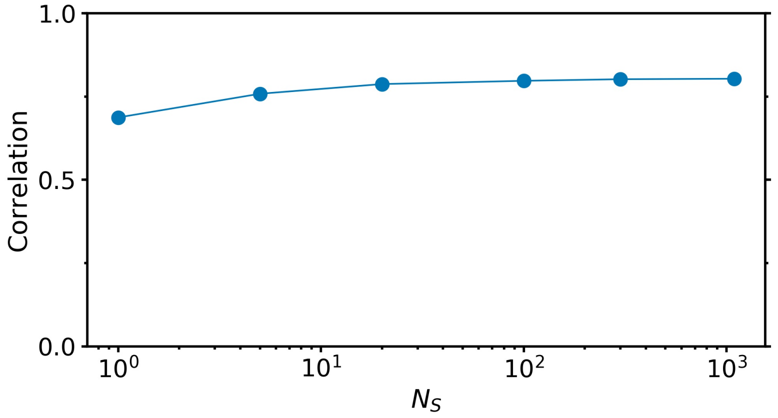


FIG. **S3**: Pearson correlation coefficient between predicted and actual propensities of the A particles of binary hard spheres at $t = \tau_\alpha$ as a function of the number of selected descriptors.

## PREDICTIVE POWER OF RADIAL AND ANGULAR DESCRIPTORS IN THE HARD-SPHERE MIXTURE

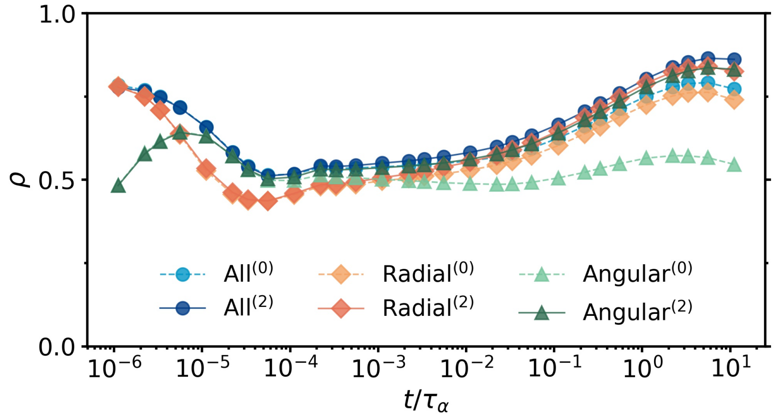


FIG. **S4**: Comparison of the Pearson correlation coefficient between predicted and actual propensities of A hard-sphere particles obtained using only radial descriptors, only angular descriptors, or both.

As in the case of the KA system, we explore the relative importance of radial and angular descriptors in the binary hard-sphere system by comparing their predictive power. To this end, we separately fit the dynamic propensity of A particles using only the radial and angular descriptors, and show the results in Fig. S4. Similar to the KA system, we find that the radial $\mathrm{LR}^{(0)}$ descriptors outperform the angular descriptors at long time scales.

## REFERENCES

[1] Kob, W. & Andersen, H. C. Testing mode-coupling theory for a supercooled binary Lennard-Jones mixture I: The van Hove correlation function. *Phys. Rev. E* **51**, 4626 (1995).
[2] Bapst, V. *et al.* Unveiling the predictive power of static structure in glassy systems. *Nat. Phys.* **16**, 448–454 (2020).
[3] Schoenholz, S. S., Cubuk, E. D., Sussman, D. M., Kaxiras, E. & Liu, A. J. A structural approach to relaxation in glassy liquids. *Nat. Phys.* **12**, 469–471 (2016).
[4] Steinhardt, P. J., Nelson, D. R. & Ronchetti, M. Bond-orientational order in liquids and glasses. *Phys. Rev. B* **28**, 784 (1983).
[5] Pedregosa, F. *et al.* Scikit-learn: Machine learning in Python. *J. Mach. Learn. Res.* **12**, 2825 (2011).

[6] Boattini, E., Bezem, N., Punnathanam, S. N., Smallenburg, F. & Filion, L. Modeling of many-body interactions between elastic spheres through symmetry functions. *J. Chem. Phys.* **153**, 064902 (2020).
